# Supplementary material for: Low-power photothermal self-oscillation of bimetallic nanowires
Source: arXiv:1610.07591 ancillary file (2016-12-28)
Supplement: Supplementary file 1 [file supplementary_info.pdf]

# Low-power photothermal self-oscillation of bimetallic nanowires
# SUPPLEMENTARY INFORMATION

Roberto De Alba,[1] T. S. Abhilash,[1] Richard H. Rand,[2,3] Harold G. Craighead,[4] and Jeevak M. Parpia[1]
[1]*Department of Physics, Cornell University, Ithaca NY, USA*
[2]*Department of Mathematics, Cornell University, Ithaca NY, USA*
[3]*Sibley School of Mechanical and Aerospace Engineering, Cornell University, Ithaca NY, USA*
[4]*School of Applied and Engineering Physics, Cornell University, Ithaca NY, USA*

---

**CONTENTS**

S1. Perturbation theory for photothermal self-oscillation 2
S2. Static nanowire behavior 7
S3. Critical power and hysteresis 8
S4. Estimation of thermal parameters 10
S5. Beam theory for supporting cantilevers 13
S6. Nonlinearity of the optical readout technique 15

## S1. PERTURBATION THEORY FOR PHOTOTHERMAL SELF-OSCILLATION

The governing equations of motion are:

$$\ddot{z} + \gamma\dot{z} + \omega_0^2(1 + CT)(z - DT) = 0 \tag{S1}$$

$$\dot{T} + \frac{1}{\tau}T = APg(z) \tag{S2}$$

$$g(z) = \alpha + \beta\sin^2\left(\frac{2\pi(z+\phi)}{\lambda} - \frac{\pi}{4}\right) \tag{S3}$$

Eqs. S1 & S2 have the static solution $z_0 = \tau DAPg(z_0)$ and $T_0 = z_0/D$. We can define a new coordinate system as deviations from this equilibrium $x = z - z_0$ and $u = T - T_0$, which leads to:

$$\ddot{x} + \gamma\dot{x} + \omega_0^2(1 + CT_0 + Cu)(x - Du) = 0 \tag{S4}$$

$$\dot{u} + \frac{1}{\tau}u = -\frac{1}{\tau}T_0 + APg(x + z_0) \tag{S5}$$

$$g(x + z_0) = \alpha + \beta\sin^2\left(\frac{2\pi(x + z_0 + \phi)}{\lambda} - \frac{\pi}{4}\right) \tag{S6}$$

where we have introduced $x_0 = \phi - z_0$. For convenience we now rescale our units of time and displacement such that the resonant frequency $\omega_0 = 1$ and laser wavelength $\lambda = 1$:

$$\ddot{x} + \frac{1}{Q}\dot{x} + (1 + CT_0 + Cu)(x - D'u) = 0 \tag{S7}$$

$$\dot{u} + \frac{1}{\tau'}u = -\frac{1}{\tau'}T_0 + A'Pg(x + z_0) \tag{S8}$$

$$g(x + z_0) = \alpha + \beta\sin^2\left(2\pi(x + z_0 + \phi) - \frac{\pi}{4}\right). \tag{S9}$$

Here the quantities $x, z_0, \phi$ are now expressed in units of $\lambda$ and we have introduced the quality factor $Q = \omega_0/\gamma$. Furthermore, we have defined $D' = D/\lambda$, $\tau' = \tau\omega_0$, and $A' = A/\omega_0$. Hereafter we will work exclusively with these rescaled parameters, and for brevity we will not write the primes.

In performing the perturbation theory, we will be required to approximate $g(x + z_0)$ by a polynomial. We choose to expand $g(x + z_0)$ in a Taylor series about $x + z_0 = -\phi$ so that the coefficients of our series are independent of $\phi$. We will truncate this series at $N + 1$ terms, and refer to the truncated series as $h(x) \approx g(x + z_0)$:

$$h(x) = \sum_{n=0}^{N} \frac{g^{(n)}(-\phi)}{n!}(x + z_0 + \phi)^n = \sum_{n=0}^{N} k_n(x + z_0 + \phi)^n \tag{S10}$$

where $g^{(n)}(-\phi)$ denotes the $n^{\text{th}}$ derivative of $g(x + z_0)$ evaluated at $x + z_0 = -\phi$. Note that if $N \to \infty$ we have $h(x) = g(x + z_0)$. The first few coefficients $k_n$ are given by:

$$\begin{aligned}
k_0 &= \alpha + \frac{\beta}{2}\\
k_1 &= -2\pi\beta\\
k_3 &= \frac{16}{3}\pi^3\beta\\
k_5 &= -\frac{64}{15}\pi^5\beta\\
k_7 &= \frac{512}{315}\pi^7\beta\\
k_n &= 0, \ \ \text{even}\, n > 0
\end{aligned} \tag{S11}$$

Thus, finally, we will seek a solution to the coupled differential equations:

$$\ddot{x} + \frac{1}{Q}\dot{x} + (1 + CT_0 + Cu)(x - Du) = 0 \tag{S12}$$

$$\dot{u} + \frac{1}{\tau}u = -\frac{1}{\tau}T_0 + APh(x) \tag{S13}$$

We will solve Eqs. S12 & S13 via the Poincaré-Lindstedt perturbation method. To do this, we must scale $1/Q, Cu$, and $Du$ by a small dimensionless parameter $\epsilon \ll 1$. This will yield solutions for $x(t)$ and $u(t)$ that are power series in $\epsilon$: $x = x_1 + x_2\epsilon + x_3\epsilon^2 + \cdots$ and $u = u_1 + u_2\epsilon + u_3\epsilon^2 + \cdots$. In order to perturbatively solve for the oscillation frequency $\omega = \omega_1 + \omega_2\epsilon + \omega_3\epsilon^2 + \cdots$ we must once more scale the time dimension by $\omega$. This leads to the coupled system:

$$\omega^2\ddot{x} + \frac{\epsilon\omega}{Q}\dot{x} + (1 + CT_0 + \epsilon Cu)(x - \epsilon Du) = 0 \tag{S14}$$

$$\omega\dot{u} + \frac{1}{\tau}u = -\frac{1}{\tau}T_0 + APh(x) \tag{S15}$$

Setting $\epsilon = 0$ gives us the lowest order of the perturbation:

$$\omega_1^2\ddot{x}_1 + (1 + CT_0)x_1 = 0 \tag{S16}$$

$$\omega_1\dot{u}_1 + \frac{1}{\tau}u_1 = -\frac{1}{\tau}T_0 + APh(x_1) \tag{S17}$$

Choosing $\omega_1^2 = 1 + CT_0$ in Eq. S16 results in the solution $x_1 = R\cos t$. This solution is now substituted into Eq. S17 to solve for $u_1$. Because $h(x_1)$ is a polynomial in $x_1$, this leads to:

$$\omega_1\dot{u}_1 + \frac{1}{\tau}u_1 = u_{10} + \sum_{n=1}^{N} u_{1n}\cos nt \tag{S18}$$

where the coefficients $u_{10}$ and $u_{1n}$ depend on $T_0$, $R$, and the details of $h(x_1)$. We will derive these coefficients on the next page, but for now we proceed assuming they are known.

Solving Eq. S18, the steady-state solution for $u_1$ is:

$$u_1(t) = \tau u_{10} + \sum_{n=1}^{N} \frac{\tau u_{1n}}{1 + n^2\omega_1^2\tau^2}(\cos nt + n\omega_1\tau\sin nt) \tag{S19}$$

Thus the time-averaged value of $u$ (to order $\epsilon^0$ in perturbation theory) increases by an amount $\tau u_{10}$ during oscillation.

We now proceed to order $\epsilon^1$ of perturbation theory by substituting $x = x_1 + \epsilon x_2$, $u = u_1 + \epsilon u_2$ and $\omega = \omega_1 + \epsilon\omega_2$ into Eq. S14 and neglecting terms of order $\epsilon^2$ and higher:

$$\epsilon\omega_1^2\ddot{x}_2 + \epsilon\omega_1^2 x_2 + 2\epsilon\omega_1\omega_2\ddot{x}_1 + \frac{\epsilon\omega_1}{Q}\dot{x}_1 - \epsilon\omega_1^2 Du_1 + \epsilon Cu_1x_1 = 0 \tag{S20}$$

Rearranging terms, this equation can be written in the more familiar form:

$$\ddot{x}_2 + x_2 = -\frac{2\omega_2}{\omega_1}\ddot{x}_1 - \frac{1}{\omega_1 Q}\dot{x}_1 + Du_1 - \frac{C}{\omega_1^2}u_1x_1 \tag{S21}$$

Thus $x_2$ represents a simple harmonic oscillator with forcing terms given by the right hand side of Eq. S21. In order for $x_2$ not to grow without bound, secular terms must be removed. In other words the forcing terms at frequency $\omega = 1$ must vanish. Thus we proceed by substituting $x_1 = R\cos t$ and Eq. S19 for $u_1$, collecting terms proportional to $\cos t$ and $\sin t$, and equating them to zero. Collecting $\sin t$ terms in Eq. S21 leads to

$$\frac{\omega_1^2 Du_{11}}{1 + \omega_1^2\tau^2} - \frac{CRu_{12}}{1 + 4\omega_1^2\tau^2} + \frac{R}{\tau^2 Q} = 0 \tag{S22}$$

which can be solved for $R$, bearing in mind that the coefficients $u_{11}$ and $u_{12}$ are dependent on $R$. Collecting $\cos t$ terms in Eq. S21 gives

$$\frac{2\tau\omega_1^2 Du_{11}}{1 + \omega_1^2\tau^2} - \frac{\tau CRu_{12}}{1 + 4\omega_1^2\tau^2} + 4R\omega_1\omega_2 - 2\tau CRu_{10} = 0 \tag{S23}$$

which can be solved for $\omega_2$ once $R$ is known.

According to Eq. S22, the oscillation amplitude $R$ is determined by the coefficients $u_{11}$ and $u_{12}$, which are the forcing terms for $u$ at frequency $\omega$ and $2\omega$ in Eq. S18. Moreover, the average temperature change is determined by $u_{10}$. We will now proceed to calculate these terms based on $h(x)$ in Eq. S17.

Deriving $u_{10}, u_{11}$, and $u_{12}$ is most easily done if we first rewrite $h(x)$ as a series in $x$ rather than $x + z_0 + \phi$. Thus we have

$$h(x) = \sum_{n=0}^{N} \frac{h_0^{(n)}}{n!} x^n \tag{S24}$$

where $h_0^{(n)}$ is the $n^{\text{th}}$ derivative of $h(x)$ evaluated at $x = 0$. Note that this Taylor series terminates at order $x^N$ because $h(x)$ is by definition an $N^{\text{th}}$ order polynomial (see Eq. S10). If we take $h(x)$ to be $7^{\text{th}}$ order, as is done in the main text, then the derivatives $h_0^{(n)}$ are related to the factors $k_n$ in Eq. S10 by:

$$\begin{aligned}
h_0^{(0)} &= k_0 + k_1 x_0 + k_3 x_0^3 + k_5 x_0^5 + k_7 x_0^7 \\
h_0^{(1)} &= k_1 + 3k_3 x_0^2 + 5k_5 x_0^4 + 7k_7 x_0^6 \\
h_0^{(2)} &= 6k_3 x_0 + 20k_5 x_0^3 + 42k_7 x_0^5 \\
h_0^{(3)} &= 6k_3 + 60k_5 x_0^2 + 210k_7 x_0^4 \\
h_0^{(4)} &= 120k_5 x_0 + 840k_7 x_0^3 \\
h_0^{(5)} &= 120k_5 + 2520k_7 x_0^2 \\
h_0^{(6)} &= 5040k_7 x_0 \\
h_0^{(7)} &= 5040k_7
\end{aligned} \tag{S25}$$

where we have defined $x_0 = z_0 + \phi$. Equating the right hand sides of Eqs. S17 & S18 then gives:

$$u_{10} + \sum_{m=1}^{N} u_{1m} \cos mt = -\frac{1}{\tau} T_0 + AP \sum_{n=0}^{N} \frac{h_0^{(n)}}{n!} x_1^n \tag{S26}$$

In order to calculate $u_{10}$, $u_{11}$, and $u_{12}$ we now substitute $x_1 = R\cos t$ and invoke the power formulas for cosines

$$\text{even } n: \qquad \cos^n t = \frac{1}{2^n}\binom{n}{n/2} + \frac{1}{2^{n-1}} \sum_{k=0}^{(n/2)-1} \binom{n}{k} \cos[(n-2k)t] \tag{S27}$$

$$\text{odd } n: \qquad \cos^n t = \frac{1}{2^{n-1}} \sum_{k=0}^{(n-1)/2} \binom{n}{k} \cos[(n-2k)t] \tag{S28}$$

where $\binom{a}{b} = a!/(b!(a-b)!)$ is a binomial coefficient. For even $n$, the constant term arising from $\cos^n t$ is simply $(1/2^n)\binom{n}{n/2}$. Furthermore, because only $\cos^n t$ with even $n$ will lead to $\cos mt$ with even $m$, the $u_{10}$ in Eq. S26 is

$$\begin{aligned}
u_{10} &= -\frac{1}{\tau} T_0 + AP \sum_{n=0,2,4,\ldots}^{N} \frac{h_0^{(n)}}{n!} \left(\frac{R}{2}\right)^n \frac{n!}{(n/2)!(n/2)!} \\
&= -\frac{1}{\tau} T_0 + AP \sum_{m=0}^{M_0} \frac{h_0^{(2m)}}{(m!)^2} \left(\frac{R}{2}\right)^{2m}
\end{aligned} \tag{S29}$$

where $M_0 = \text{floor}(N/2)$. The value of $u_{10}$ can similarly be found by substituting Eq. S28 into Eq. S26 with $n - 2k = 1$. Only odd $n \geq 1$ contribute to this sum. This gives

$$\begin{aligned}
u_{11} &= AP \sum_{n=1,3,5,\ldots}^{N} \frac{h_0^{(n)}}{n!} \left(\frac{R^n}{2^{n-1}}\right) \frac{n!}{(\frac{n-1}{2})!(\frac{n+1}{2})!} \\
&= 2AP \sum_{m=0}^{M_1} \frac{h_0^{(2m+1)}}{m!(m+1)!} \left(\frac{R}{2}\right)^{2m+1}
\end{aligned} \tag{S30}$$

where $M_1 = \text{floor}((N-1)/2)$. Lastly, $u_{12}$ is found by substituting $n - 2k = 2$ into Eq. S27 and Eq. S26. Only even $n \geq 2$ contribute to this sum:

$$\begin{aligned} u_{12} &= AP \sum_{n=2,4,6,\ldots}^{N} \frac{h_0^{(n)}}{n!} \left(\frac{R^n}{2^{n-1}}\right) \frac{n!}{(\frac{n}{2}-1)!(\frac{n}{2}+1)!} \\ &= 2AP \sum_{m=0}^{M_2} \frac{h_0^{(2m+2)}}{m!(m+2)!} \left(\frac{R}{2}\right)^{2m+2} \end{aligned} \tag{S31}$$

where $M_2 = \text{floor}((N-2)/2)$. Interestingly, if we take $N \to \infty$ these sums bear remarkable resemblance to modified Bessel functions of the first kind:

$$I_\alpha(x) = \sum_{m=0}^{\infty} \frac{1}{m!(m+\alpha)!} \left(\frac{x}{2}\right)^{2m+\alpha} \tag{S32}$$

Thus for the case of $N \to \infty$ we may write $u_{10} \ldots u_{12}$ as:

$$u_{10} = -\frac{1}{\tau} T_0 + API_0 \left(R \frac{d}{dx}\right) \cdot h(x)\Big|_{x=0} \tag{S33}$$

$$u_{11} = 2API_1 \left(R \frac{d}{dx}\right) \cdot h(x)\Big|_{x=0} \tag{S34}$$

$$u_{12} = 2API_2 \left(R \frac{d}{dx}\right) \cdot h(x)\Big|_{x=0} \tag{S35}$$

In fact, it can be shown that for all $n > 0$ the temperature variation at frequency $n\omega$ is given by:

$$u_{1n} = 2API_n \left(R \frac{d}{dx}\right) \cdot h(x)\Big|_{x=0} \tag{S36}$$

Of course, in the $N \to \infty$ limit we also have $h(x) = g(x + z_0)$.

If we truncate $h(x)$ at $N = 7$, then we have $M_0 = 3$ in Eq. S29. Therefore by Eq. S18, the time-averaged change in temperature is given by:

$$\tau u_{10} = -T_0 + \tau AP \sum_{m=0}^{3} \frac{h_0^{(2m)}}{(m!)^2} \left(\frac{R}{2}\right)^{2m} \tag{S37}$$

Furthermore, when $N = 7$ we have $M_1 = 3$ and $M_2 = 2$ in Eqs. S30 & S31. Thus $u_{11}$ contains all odd powers of $R$ from $R^1$ to $R^7$, and $u_{12}$ contains all even powers from $R^2$ to $R^6$. Upon substituting $u_{11}$ and $u_{12}$ into Eq. S22, we then finally arrive at our equation for $R$:

$$0 = c_0 + c_1 R^2 + c_2 R^4 + c_3 R^6 \tag{S38}$$

where

$$\begin{aligned} c_0 &= \frac{\omega_1^2 D}{1+\omega_1^2\tau^2} h_0^{(1)} + \frac{1}{\tau^2 APQ} \\ c_1 &= \frac{\omega_1^2 D}{1+\omega_1^2\tau^2} \frac{h_0^{(3)}}{2^2 1!2!} - \frac{C}{1+4\omega_1^2\tau^2} \frac{h_0^{(2)}}{2^1 0!2!} \\ c_2 &= \frac{\omega_1^2 D}{1+\omega_1^2\tau^2} \frac{h_0^{(5)}}{2^4 2!3!} - \frac{C}{1+4\omega_1^2\tau^2} \frac{h_0^{(4)}}{2^3 1!3!} \\ c_3 &= \frac{\omega_1^2 D}{1+\omega_1^2\tau^2} \frac{h_0^{(7)}}{2^6 3!4!} - \frac{C}{1+4\omega_1^2\tau^2} \frac{h_0^{(6)}}{2^5 2!4!} \end{aligned}$$

The results shown above are expressed in dimensionless units. When re-dimensionalized, they reproduce Eq. 5 of the main text. The $\epsilon^1$-order correction to the resonant frequency is (upon rearranging Eq. S23)

$$\omega_2 = \frac{\tau C}{2\omega_1} u_{10} - \frac{\omega_1 \tau D}{1+\omega_1^2\tau^2} \frac{u_{11}}{2R} + \frac{\tau C}{1+4\omega_1^2\tau^2} \frac{u_{12}}{4\omega_1} \tag{S39}$$

When $h(x)$ is truncated at $N = 7$ this becomes

$$\omega_2 = d_0 + d_1 R^2 + d_2 R^4 + d_3 R^6 \tag{S40}$$

where (again in dimensionless units)

$$\begin{aligned}
d_0 &= -\frac{\omega_1 \tau D}{1+\omega_1^2\tau^2}\,\frac{APh_0^{(1)}}{2^1 0!1!} + \frac{\tau C}{2\omega_1}\left(-\frac{1}{\tau}T_0 + APh_0^{(0)}\right)\\
d_1 &= -\frac{\omega_1 \tau D}{1+\omega_1^2\tau^2}\,\frac{APh_0^{(3)}}{2^3 1!2!} + \frac{\tau C}{1+4\omega_1^2\tau^2}\,\frac{APh_0^{(2)}}{2^3 0!2!\omega_1}\\
d_2 &= -\frac{\omega_1 \tau D}{1+\omega_1^2\tau^2}\,\frac{APh_0^{(5)}}{2^5 2!3!} + \frac{\tau C}{1+4\omega_1^2\tau^2}\,\frac{APh_0^{(4)}}{2^5 1!3!\omega_1}\\
d_3 &= -\frac{\omega_1 \tau D}{1+\omega_1^2\tau^2}\,\frac{APh_0^{(7)}}{2^7 3!4!} + \frac{\tau C}{1+4\omega_1^2\tau^2}\,\frac{APh_0^{(6)}}{2^7 2!4!\omega_1}
\end{aligned}$$

## S2. STATIC NANOWIRE BEHAVIOR

From Eqs. S1 & S2 the static nanowire must satisfy

$$z_0 = DT_0 \tag{S41}$$

$$\frac{1}{\tau}T_0 = \tau APg(z_0) \tag{S42}$$

Rearranging these shows that the nanowire equilibrium is determined by the roots of the following equation:

$$0 = APg(z_0) - \frac{z_0}{\tau D} \tag{S43}$$

Near $P = 0$ this equation has only one root, but as $P$ increases more roots develop. This function is plotted for multiple $P$ values in Fig. S1 (a) for $\phi = 0$. The upper panel displays the lowest valid solution of Eq. S43, which has a discontinuous jump in $z_0$ from one crest of $g(z)$ to the next as $P$ increases quasi-statically. These results suggest that for high enough $P$ values, $z_0$ will reside only in regions of $g(z)$ with negative slope $dg/dz$ – i.e. in regions conducive to self-oscillation. It should be noted that in this experiment (and in the function plotted in Fig. S1), a positive $D$ value is assumed. In an experiment where $D < 0$, the equilibrium $z_0$ would shift towards negative values for increasing $P$, and the tendency of $z_0$ to reside only in regions conducive to self-oscillation (regions of positive $dg/dz$ in this case) would still be observed.

Fig. S1 (b-d) show the expected equilibrium position for our nanowire based on Eq. S43 for varying $\phi$ and $P$ values. Fig. S1 (b) displays the equilibrium shift relative to the $P = 0$ position (i.e. $z_0$), which is periodic in $\lambda/2$ as expected. Fig. S1 (c) displays the absolute nanowire position within the standing wave (i.e. $z_0 + \phi$), and the slope $dg/dz$ at this absolute position is shown in Fig. S1 (d). The latter clearly indicates that above $P \approx 50\,\mu$W the nanowire is most likely to be found in a region with negative $dg/dz$.

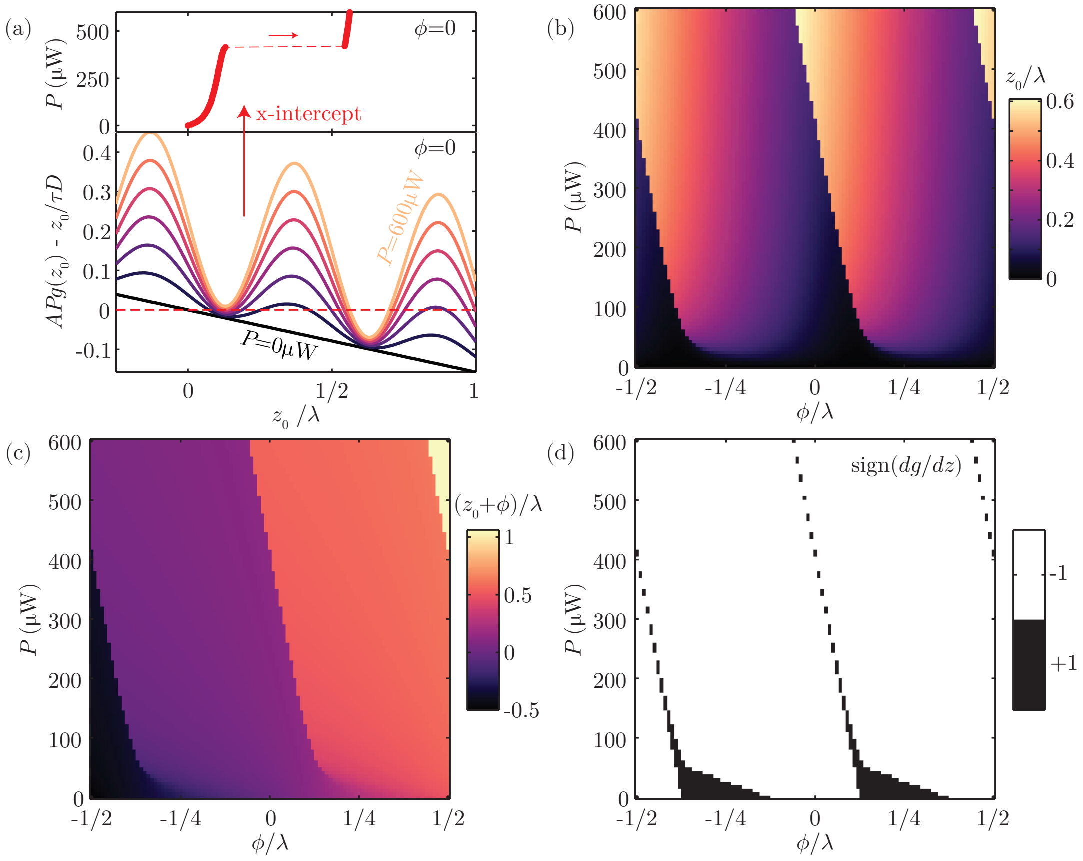


FIG. S1. Equilibrium position of the static nanowire vs laser power $P$ and initial position $\phi$

## S3. CRITICAL POWER AND HYSTERESIS

Reproducing a result from Section S1, the amplitude $R$ of self-oscillation is (in dimensionful units):

$$0 = c_0 + c_1 R^2 + c_2 R^4 + c_3 R^6 \tag{S44}$$

where

$$c_0 = \frac{\omega_1^2 D}{1+\omega_1^2\tau^2} g_{z_0}^{(1)} + \frac{\gamma}{\tau^2 AP}$$
$$c_1 = \frac{\omega_1^2 D}{1+\omega_1^2\tau^2} \frac{g_{z_0}^{(3)}}{2^2 1!2!} - \frac{\omega_0^2 C}{1+4\omega_1^2\tau^2} \frac{g_{z_0}^{(2)}}{2^1 0!2!}$$
$$c_2 = \frac{\omega_1^2 D}{1+\omega_1^2\tau^2} \frac{g_{z_0}^{(5)}}{2^4 2!3!} - \frac{\omega_0^2 C}{1+4\omega_1^2\tau^2} \frac{g_{z_0}^{(4)}}{2^3 1!3!}$$
$$c_3 = \frac{\omega_1^2 D}{1+\omega_1^2\tau^2} \frac{g_{z_0}^{(7)}}{2^6 3!4!} - \frac{\omega_0^2 C}{1+4\omega_1^2\tau^2} \frac{g_{z_0}^{(6)}}{2^5 2!4!}$$

Here we have made the approximation $h(x) = g(x + z_0)$. This can be rearranged to express $P$ as a function of $R$:

$$P = \frac{-\gamma/(\tau^2 A)}{b + c_1 R^2 + c_2 R^4 + c_3 R^6} \tag{S45}$$

where $b = (\omega_1^2 D g_{z_0}^{(1)})/(1+\omega_1^2\tau^2)$. The critical laser power $P_{\text{crit}}$ is simply the $R = 0$ value of this function:

$$P_{\text{crit}} = -\frac{\gamma\left(1+\omega_1^2\tau^2\right)}{\omega_1^2\tau^2 D A g_{z_0}^{(1)}} \tag{S46}$$

Whether the transition to self-oscillation will be hysteretic or non-hysteretic (i.e. whether the Hopf bifurcation will be subcritical or supercritical) is determined by the curvature $d^2P/dR^2$ at $R = 0$. Upon differentiating Eq. S45 twice, one finds that this curvature is given by

$$\left.\frac{d^2P}{dR^2}\right|_{R=0} = \frac{2\gamma c_1}{\tau^2 A b^2} \tag{S47}$$

Because physical values of $\gamma$ and $A$ must be positive, this result suggests that $c_1 < 0$ is the necessary condition for a hysteretic transition. Such a transition is depicted in Fig. S2. The parameters used to produce this figure are identical to the experimental values of our nanowire, except $C$ has been increased by a factor of 100; $\phi$ is near $\lambda/8$, where $|g_{z_0}^{(2)}|$

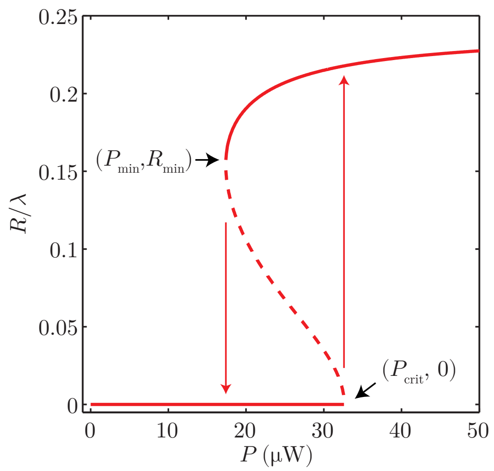


FIG. S2. A subcritical Hopf bifurcation. A dashed line indicates unstable behavior.

is maximal. In this figure $z_0$ (the time-averaged position) has been held fixed over the entire $P$ range to simplify the results.

The width of the hysteresis region can be found by analyzing the first derivative of $P$:

$$\frac{dP}{dR} = \frac{\gamma}{\tau^2 A} \frac{2c_1 R + 4c_2 R^3 + 6c_3 R^5}{(b + c_1 R^2 + c_2 R^4 + c_3 R^6)^2} \tag{S48}$$

As seen in Fig. S2, the minimum $P$ value at which self-oscillation is sustainable coincides with a turning point in $P(R)$ – i.e. it occurs when $dP/dR = 0$. Note that $dP/dR = 0$ also occurs at $R = 0$ – i.e. at the critical power $P = P_{\text{crit}}$. The lower edge of the self-oscillation region is thus found by solving the following equation for the minimum amplitude $R_{\text{min}}$

$$0 = 2c_1 + 4c_2 R^2 + 6c_3 R^4 \tag{S49}$$

and substituting the resulting value back into Eq. S45 for $P$ to give $P_{\text{min}} = P(R_{\text{min}})$. This calculation seems straightforward if $c_1, c_2$, and $c_3$ are taken as constants, but in actuality these quantities are dependent on $z_0$, which generally depends on $P$; this makes calculation of $P_{\text{min}}$ much more difficult. Therefore one approach to calculating $P_{\text{min}}$ would be to iteratively solve Eqs. S49, S45 & S43 for $R$, $P$, and $z_0$ until they converge on fixed values.

## S4. ESTIMATION OF THERMAL PARAMETERS

The mechanical and thermal parameters of our system $(\omega_0, \tau, C, D)$ can be accurately estimated by knowledge of the material composition of our nanowire and the cantilevers by which it is suspended. The optical parameters $(A, \alpha, \beta)$ require also knowledge of our laser spot size and the refractive index of the reflective silicon back-plane.

The resonant frequency of a tensioned wire composed of a single material with Young's modulus $E$ and internal strain $\varepsilon$ is

$$\omega_0 = \frac{\pi}{L}\sqrt{\frac{E\varepsilon}{\rho}} \tag{S50}$$

where $L$ is the wire length and $\rho$ is the mass per unit volume. This equation neglects terms due to bending of the wire, and is valid only in the high tension limit. For a wire composed of two distinct materials, this becomes

$$\omega_0 = \frac{\pi}{L}\sqrt{\frac{\sigma_{\mathrm{tot}}}{\mu_{\mathrm{tot}}}} = \frac{\pi}{L}\sqrt{\frac{E_1 A_1 \varepsilon_1 + E_2 A_2 \varepsilon_2}{\rho_1 A_1 + \rho_2 A_2}} \tag{S51}$$

where $\sigma_{\mathrm{tot}}$, $\mu_{\mathrm{tot}}$ are the total tensile force and mass per unit length of the wire. The subscripts $1, 2$ have been used to distinguish between the two materials and $A_n$ is the cross-sectional area of either material.

The parameter $C$, which denotes the fractional frequency change per unit temperature in Eq. S1 can be approximated by

$$C = \frac{1}{\sigma_{\mathrm{tot}}}\left(\frac{d\sigma_{\mathrm{tot}}}{dT}\right) \approx -\frac{E_1 A_1 \alpha_1 + E_2 A_2 \alpha_2}{E_1 A_1 \varepsilon_1 + E_2 A_2 \varepsilon_2} \tag{S52}$$

Here $\alpha_n$ is the linear thermal expansion coefficient of material $n$, and this effect is entirely attributed to tension change within the wire. We have assumed here that as the temperature changes both materials are free to expand and do not influence one another. This is not entirely physical (especially for large $T$), but we will see that this rough approximation agrees well with the experimentally measured value.

The parameter $D$ describes coupling between temperature and the vertical position of our nanowire. This coupling is caused by the bimetalic cantilevers on either end of the nanowire, which at room temperature ($\approx 300\,\mathrm{K}$) curve upward due to unbalanced stresses between the Nb film (top layer) and the underlying SiN. A detailed calculation of $D$ based on cantilever dimensions is presented in Section S5. Here we estimate $D$ for a single nanowire based on angled-SEM (Scanning Electron Microscopy) measurements of the cantilever length $l_c$ and equilibrium angle $\theta$ above the horizontal. If $\theta$ is known, an estimate for $D$ can be obtained by modeling the cantilever as acting under the influence of an internal torque $\mathcal{T}_c$ which pulls it up and nanowire tension $\sigma_{\mathrm{tot}}$ which pulls it along the horizontal. Relative to a rotation axis at the cantilever clamped edge, the torque exerted by the nanowire is $\sigma_{\mathrm{tot}} l_c \sin\theta$; in equilibrium we must therefore have $\mathcal{T}_c = \sigma_{\mathrm{tot}} l_c \sin\theta$. The vertical position of the cantilever free end is $z = l_c \sin\theta$. If the two cantilevers supporting the nanowire have differing lengths $l_{c1}, l_{c2}$ and equilibrium angles $\theta_{c1}, \theta_{c2}$, then the vertical position of the nanowire center is:

$$z = \frac{l_{c1}\sin\theta_{c1} + l_{c2}\sin\theta_{c2}}{2} = \frac{\mathcal{T}_{c1} + \mathcal{T}_{c2}}{2\sigma_{\mathrm{tot}}} \tag{S53}$$

The change in vertical position of the nanowire per unit temperature change is then

$$D \approx -\left(\frac{\mathcal{T}_{c1} + \mathcal{T}_{c2}}{2\sigma_{\mathrm{tot}}^2}\right)\left(\frac{d\sigma_{\mathrm{tot}}}{dT}\right) \approx \left(\frac{\mathcal{T}_{c1} + \mathcal{T}_{c2}}{2}\right)\frac{E_1 A_1 \alpha_1 + E_2 A_2 \alpha_2}{\left(E_1 A_1 \varepsilon_1 + E_2 A_2 \varepsilon_2\right)^2} \tag{S54}$$

This formula holds only for small deviations away from the equilibrium angles $\theta_{c1}, \theta_{c2}$. As with $C$, this parameter is proportional to the change in total wire tension per unit temperature.

For a heated mechanical resonator composed of a single material, the thermal time constant $\tau$ would simply be:

$$\tau = \frac{L_{\mathrm{eff}}}{\Lambda A_{\mathrm{eff}}}\,\rho c V_{\mathrm{eff}} \tag{S55}$$

where $\Lambda, c$ are the thermal conductivity and specific heat of the material, and $L_{\mathrm{eff}}, A_{\mathrm{eff}}$ are the effective length and cross section of the conductive channel. $V_{\mathrm{eff}}$ is the effective volume of heated material, and the combination $\rho c V_{\mathrm{eff}}$ is the thermal mass. The combination $L_{\mathrm{eff}}/(\Lambda A_{\mathrm{eff}})$ is the thermal resistance.

In our system, heat flows from the nanowire midpoint (where the laser is focused) out to the clamped edges of the two cantilevers. It flows in parallel paths through the SiN (material 1) and Nb (material 2), along two possible directions out from the midpoint. The thermal resistance of the nanowire (from midpoint to endpoint) is $R_w = (1/2)L/(\Lambda_1 A_1 + \Lambda_2 A_2)$. The resistance of either cantilever is $R_c = l_c/(\Lambda_1 A_{c1} + \Lambda_2 A_{c2})$. Because of the two directions outward from the midpoint, the total resistance is $R_{\rm tot} = (R_w + R_c)/2$. The total thermal mass $\mu$ of the system (assuming cantilevers of equal length $l$) is given by $\mu_{\rm tot} = c_1\rho_1(LA_1 + 2l_cA_{c1}) + c_2\rho_2(LA_2 + 2l_cA_{c2})$. Therefore the thermal time is

$$\tau = \mu_{\rm tot} R_{\rm tot} \tag{S56}$$

The $A$ parameter in Eq. S2 can be expressed as:

$$A = \frac{a}{\mu_{\rm tot}} = \frac{[1 - \exp(-4\pi k_{Nb} t_{Nb}/\lambda)]\,\mathrm{erf}\left(\sqrt{2}\,w/d_L\right)}{\mu_{\rm tot}} \tag{S57}$$

Here, $a$ denotes the fraction of local laser light absorbed by the nanowire; $k_{Nb}, t_{Nb}$ are the extinction coefficient and thickness of the Nb film, and $w$ is the width of the nanowire. The diameter of our Gaussian laser beam is denoted by $d_L$, and the error function $\mathrm{erf}(\sqrt{2}w/d_L)$ represents the fraction of laser beam cross-sectional area that is covered by the thin nanowire (assuming it lies along the center of the laser beam). The terms in square brackets denote the fraction of light within that thin area that is absorbed by the Nb film.

The nanowire sits in an optical standing wave generated by interference between incident light from our laser and light reflected from the silicon backplane. If we approximate the light as plane waves, it can be shown that in the presence of such a reflector the optical intensity varies with distance as

$$P(z) = P_0(1 - \sqrt{R_0})^2 + 4P_0\sqrt{R_0}\sin^2\frac{2\pi z}{\lambda} \tag{S58}$$

where $P_0$ corresponds to the incident laser power and $R_0$ is the reflection coefficient. Note that $P(z)$ here denotes the total energy density $P(z) = |\vec{E}(z)|^2$ of the light in plane $z$, where $\vec{E}$ is the combined electric field of the incident and reflected beams. Similarly, $P_0 = |\vec{E}_0|^2$ for the incident beam.

This is related to the index of refraction of the silicon, $n_{Si} = 3.83$ at 660 nm, by

$$R_0 = \left|\frac{n_{Si} - 1}{n_{Si} + 1}\right|^2 \tag{S59}$$

Thus the two remaining parameters in Eq. S2 are given by

$$\alpha = (1 - \sqrt{R_0})^2 \tag{S60}$$

$$\beta = 4\sqrt{R_0} \tag{S61}$$

Because the nanowire is much thinner than both the wavelength $\lambda$ and spot size $R_L$, we have assumed that it does not greatly affect the optical standing wave in Eq. S58.

Table S1 lists the relevant material properties for SiN and Nb. Tables S2 & S3 list the resulting mechanical and thermal parameters of our system. In Table S2, all values have been measured experimentally except for those marked with asterisks (*), which were calculated based on Eq. S51. In Table S3, $A$ excludes the error function shown in Eq. S57 since $d_L$ (the laser spot diameter) was used as a fit parameter during the experiment. The other fit parameters were $1/\tau$ (the cooling rate) and $\phi$, the initial position of the nanowire within the optical field, as seen in Eq. S3. Typical $d_L$ values arising from the fits were $2\mu$m to $2.5\mu$m.

| | SiN | Nb | Units | Description |
|---|---|---|---|---|
| $\rho$ | 3000 | 8600 | $\mathrm{kg\,m^{-3}}$ | mass density |
| $Y$ | 290 | 105 | GPa | Young's modulus |
| $\alpha$ | 3 | 7 | $10^{-6}\,\mathrm{K^{-1}}$ | thermal expansion coeff. |
| $\Lambda$ | 22 | 54 | $\mathrm{Wm^{-1}K^{-1}}$ | thermal conductivity |
| $c$ | 700 | 265 | $\mathrm{Jkg^{-1}K^{-1}}$ | specific heat |
| $k$ | 0 | 3.36 | | extinction coefficient |

TABLE S1. Material parameters used for SiN & Nb

| | Value | Units | Description |
|---|---|---|---|
| $\omega_0/2\pi$ | 3.03 | MHz | frequency |
| $A_1$ | 875 | $\mathrm{nm^2}$ | wire SiN cross-section |
| $A_2$ | 1420 | $\mathrm{nm^2}$ | wire Nb cross-section |
| $\varepsilon_{\mathrm{SiN}}$ | 0.3 | % | *strain |
| $\varepsilon_{\mathrm{Nb}}$ | 0.02 | % | *strain |
| $t_{\mathrm{Nb}}$ | 20 | nm | Nb thickness |
| $w$ | 51 | nm | wire width |
| $L$ | 40 | $\mu$m | wire length |
| $l_{c1}$ | 2.4 | $\mu$m | cantilever length |
| $l_{c2}$ | 4.1 | $\mu$m | cantilever length |
| $\theta_1$ | 16° | | cantilever angle |
| $\theta_2$ | 11° | | cantilever angle |
| $A_{c1}$ | 1.41 | $10^{-13}\,\mathrm{m^2}$ | cantilever SiN cross-section |
| $A_{c2}$ | 1.13 | $10^{-13}\,\mathrm{m^2}$ | cantilever Nb cross-section |

TABLE S2. Mechanical parameters of our nanowire

| | Theoretical Value | Value From Fit | Units |
|---|---|---|---|
| $A$ | 1.87 | – | $10^{11}\,\mathrm{K\,J^{-1}}$ |
| $1/\tau$ | 2.49 | 7.46 | kHz |
| $C$ | -2.21 | – | $10^{-3}\,\mathrm{K^{-1}}$ |
| $D$ | 1.64 | – | $\mathrm{nm\,K^{-1}}$ |
| $\alpha$ | 0.171 | – | |
| $\beta$ | 2.344 | – | |

TABLE S3. Photo-thermal parameters of our nanowire

## S5. BEAM THEORY FOR SUPPORTING CANTILEVERS

The supporting cantilevers at either end of our nanowire are composed of a layer of stressed SiN coated with a thin film (20 nm) of Nb. The Nb was deposited by sputter deposition. In this section we assume that the unbalanced stresses which cause the cantilevers to curl upward are entirely thermally induced – i.e. arising due to differing thermal expansion coefficients in the two layers and deposition of Nb atoms at a temperature $\gg 300\,\mathrm{K}$. Internal stresses in the sputtered film can also contribute to the overall stress, but will not affect the scaling of our coupling constant $D$ with cantilever dimensions.

We begin by calculating the neutral axis of a two-material composite beam. It is located a distance $\bar{y}$ above the bottom surface of the lower material (material 2). During bending, the stresses above and below the neutral axis must balance to zero. For two homogeneous materials (moduli $E_1, E_2$) of equal width and uniform thicknesses $h_1, h_2$, this condition simplifies to $0 = E_1 h_1 y_1 + E_2 h_2 y_2$. Here $y_1 = h_2 + h_1/2 - \bar{y}$ and $y_2 = h_2/2 - \bar{y}$ are the distances from the centers of materials 1 and 2 to the neutral axis. The neutral axis is therefore located at:

$$\bar{y} = \frac{\left(h_2 + \frac{h_1}{2}\right)\frac{E_1}{E_2}h_1 + \frac{1}{2}h_2^2}{\frac{E_1}{E_2}h_1 + h_2} \tag{S62}$$

This is depicted in Fig. S3. A simplification we can make in analyzing the composite beam is to use an equivalent area to represent the increased stiffness of material 1 (the Nb). This is also depicted in Fig. S3. Both materials are now assumed to have modulus $E_2$, but the top material has an effective width $bE_1/E_2$ compared to the original $b$. The area moment of inertia of the beam relative to this axis is:

$$I = \bar{I}_1 + \bar{A}_1 y_1^2 + \bar{I}_2 + \bar{A}_2 y_2^2 \tag{S63}$$

where

$$\bar{I}_1 = \frac{E_1}{E_2}\frac{bh_1^3}{12} \qquad \bar{I}_2 = \frac{bh_2^3}{12}$$
$$\bar{A}_1 = \frac{E_1}{E_2}bh_1 \qquad \bar{A}_2 = bh_2$$

Above $\bar{I}_1, \bar{I}_2$ are the moments of inertial relative to the center axes of the two materials, and the parallel axis theorem has been applied. Because we have used $E_2$ as the reference modulus, the bending stiffness of the composite beam is

$$K = E_2 I. \tag{S64}$$

In the absence of tensile force from the nanowire, either cantilever should have constant curvature $\kappa$ due to its internal/thermal stresses. Approximating this curvature by $\kappa = d^2z/dx^2$, where $z(x)$ is the vertical position of the cantilever a distance $x$ from its clamping point, leads to a deflection profile of $z(x) = (1/2)\kappa x^2$. Therefore the height of the cantilever end is $z_{\max} = (1/2)\kappa l_c^2$, where $l_c$ is the cantilever length. If the curvature is entirely thermally-induced, it is given by:

$$\kappa = \frac{6E_1E_2(h_1+h_2)h_1h_2(\alpha_1-\alpha_2)\Delta T}{E_1^2h_1^4 + 4E_1E_2h_1^3h_2 + 6E_1E_2h_1^2h_2^2 + 4E_1E_2h_1h_2^3 + E_2^2h_2^4} \tag{S65}$$

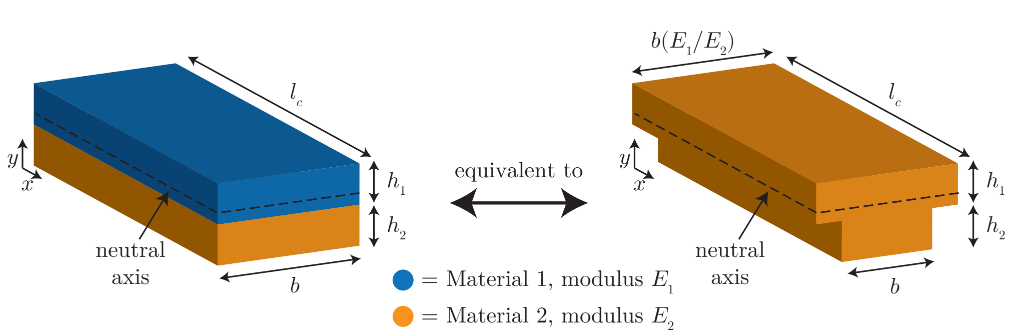


FIG. S3. Equivalent views of the composite cantilever according to beam theory

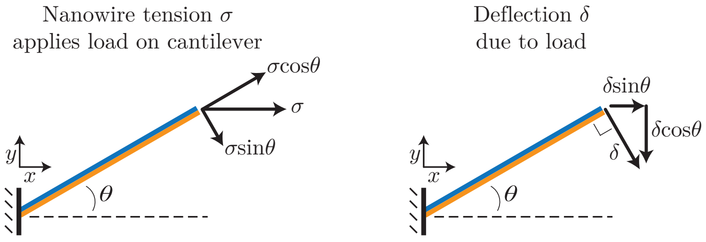


FIG. S4. Behavior of the composite beam under load

where $\alpha_1, \alpha_2$ are the thermal expansion coefficients of the two materials and $\Delta T$ is the temperature change relative to a reference temperature (the Nb deposition temperature). Other internal stresses in the two materials may contribute to $\kappa$, however, so the remaining equations will be presented for a general $\kappa$.

Shown in Fig. S4 is the effect of nanowire tension $\sigma$ on the composite beam. Here we approximate the curved cantilever as a straight beam at angle $\theta$. This allows straightforward calculation of the cantilever deflection $\delta$ due to loading by the nanowire tension. The angle $\theta$ is given by $\tan\theta = z_{\max}/l_c = \kappa l_c/2$, and the nanowire tension applies a load perpendicular to the beam of $\sigma\sin\theta$. The deflection of the composite beam is therefore

$$\delta = \frac{l_c^3 \sigma \sin\theta}{3K} \tag{S66}$$

The deflection of the cantilever end in the vertical direction is given by $\delta\cos\theta$. Thus we arrive finally at the change in vertical position per unit temperature change (i.e. stress change) of the nanowire:

$$D = \frac{d(\delta\cos\theta)}{dT} = \frac{l_c^3 \sin\theta\cos\theta}{3K}\frac{d\sigma}{dT} \tag{S67}$$

Because the bending stiffness (given by Eq. S64) $K \propto b$, where $b$ is the cantilever width, this derivation reveals that the photothermal coupling $D \propto l_c^3/b$. This suggests that $D$ can be drastically enhanced simply by using longer cantilevers. Moreover, the optimal cantilever angle is $\theta = 45^\circ$.

## S6. NONLINEARITY OF THE OPTICAL READOUT TECHNIQUE

The motion of our nanowire is detected by measuring the intensity of laser light reflected from the sample. This reflection comes from the underlying Si back-plane, and is modulated by the absorption of our nanowire. We assume that the nanowire is sufficiently thin compared to the laser wavelength ($\lambda = 660\,\text{nm}$) and spot size (Gaussian beam diameter $d_L \approx 2\,\mu\text{m}$) that it does not cause significant reflections itself or trap any light between the nanowire and mirror as in an optical cavity. Indeed, the $\sim 50\,\text{nm}$-wide nanowire acts as a single slit causing any reflected laser light to diffract away from the optical axis quite rapidly.

The power measured by our high-speed photo-detector can be approximated by $P - P_{\text{abs}}(z)$, where $P$ is the incident laser power and $P_{\text{abs}}(z)$ is the position-dependent power absorbed by our nanowire. As shown in Eq. S57, the absorbed power is

$$P_{\text{abs}}(z) = aPg(z) \tag{S68}$$

where $a$ describes the absorptive properties of the Nb film on our nanowire. The dimensionless optical intensity profile $g(z)$ (reproduced form Eq. S3) is:

$$g(z) = \alpha + \beta \sin^2\left(\frac{2\pi(z+\phi)}{\lambda} - \frac{\pi}{4}\right) \tag{S69}$$

where $\alpha, \beta$ are constants, $\phi$ is the nanowire's initial location within the optical field. The voltage generated by our photo-detector is therefore

$$V(t) = bGP[1 - ag(z(t))] \tag{S70}$$

where $b$ denotes any optical losses between the nanowire and the photo-detector (e.g. reflections at air-lens interfaces), and $G$ is the photo-detector gain.

The nonlinear relationship between $z(t)$ and $V(t)$ generates harmonics of the nanowire oscillation frequency $\omega$ in the detected voltage. The strength of these harmonics can be calculated in an analogous fashion to the terms $(u_{11}, u_{12}, \cdots)$ in Section S1. To do this, the nanowire motion is again modeled by $z = x + z_0$, where $x = R\cos\omega t$ describes the oscillation (with amplitude $R$ and frequency $\omega$) and $z_0$ is the equilibrium position.

If the optical field $g(x + z_0)$ is approximated by an $N^{\text{th}}$ order polynomial (see Eq. S10) $h(x) \approx g(x + z_0)$, then the voltage detected at frequency $i\omega$ (where $i$ is a positive integer) has amplitude

$$V_{i\omega} = -2abGP \sum_{m=0}^{M_i} \frac{h_0^{(2m+i)}}{m!(m+i)!}\left(\frac{R}{2}\right)^{2m+i} \tag{S71}$$

Here $h_0^{(n)}$ is the $n^{\text{th}}$ derivative of $h(x)$ evaluated at $x = 0$ or, equivalently, the $n^{\text{th}}$ derivative of $g(z)$ evaluated at $z = z_0$. The summation above terminates at $M_i = \text{floor}((N - i)/2)$, where $N$ is again the polynomial order or $h(x)$. See Eqs. S26 - S31 for details on the derivation.

If we take $N = 7$, the first three harmonics are given by:

$$V_{1\omega} = -2abGP\left[\frac{h_0^{(1)}}{0!1!}\left(\frac{R}{2}\right) + \frac{h_0^{(3)}}{1!2!}\left(\frac{R}{2}\right)^3 + \frac{h_0^{(5)}}{2!3!}\left(\frac{R}{2}\right)^5 + \frac{h_0^{(7)}}{3!4!}\left(\frac{R}{2}\right)^7\right] \tag{S72}$$

$$V_{2\omega} = -2abGP\left[\frac{h_0^{(2)}}{0!2!}\left(\frac{R}{2}\right)^2 + \frac{h_0^{(4)}}{1!3!}\left(\frac{R}{2}\right)^4 + \frac{h_0^{(6)}}{2!4!}\left(\frac{R}{2}\right)^6\right] \tag{S73}$$

$$V_{3\omega} = -2abGP\left[\frac{h_0^{(3)}}{0!3!}\left(\frac{R}{2}\right)^3 + \frac{h_0^{(5)}}{1!4!}\left(\frac{R}{2}\right)^5 + \frac{h_0^{(7)}}{2!5!}\left(\frac{R}{2}\right)^7\right] \tag{S74}$$

The derivatives $h_0^{(n)}$ are listed in Eq. S25. Note that the odd harmonics of $V$ only contain odd derivatives of $h(x)$ while the even harmonics only contain even derivatives. This suggests that odd harmonics of $V$ vanish when $z_0$ is located at an extremum in $g(x + z_0)$, while even harmonics vanish when $z_0$ is at an inflection point in $g(x + z_0)$. Also note that for low laser powers, when the nanowire is not undergoing self-oscillation, small-amplitude motion $R \ll \lambda$ results in the linear relationship $V_{1\omega} \approx -abGPh_0^{(1)}R$ and $V_{2\omega} \approx V_{3\omega} \approx 0$. This linear relation between the vibration amplitude $R$ and detected voltage $V_{1\omega}$ allows us to measure Lorentzian lineshapes upon driving nanowire motion inertially, as is shown in Fig. 1 (c) of the main text.
